# Supplementary material for: Towards a Fully Abstract Compiler Using Micro-Policies: Secure Compilation for Mutually Distrustful Components
Source: arXiv:1510.00697 source file (2015-10-02)
Supplement: Supplementary file 1 [file appendix.tmp.tex]

%\ottall
